# Supplementary material for: Hyperbolic Metamaterials with Bragg Polaritons
Source: arXiv:1409.3009 source file (2015-01-12)
Supplement: Supplementary file 1 [file Suppl20150112.pdf]

# Supplemental material: Hyperbolic Metamaterials with Bragg Polaritons

## I. BRAGG MIRROR MODEL. EIGENMODE EQUATION

We consider the Bragg mirror shown in Fig. S1. The structure consists of the periodic array of the alternating dielectric layers with the quantum wells (QWs) placed in the centres of one type of the layers.

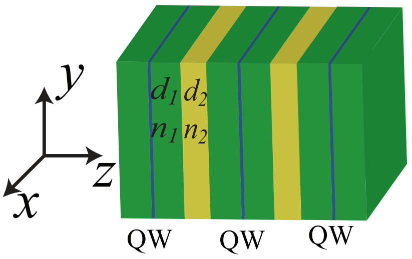


Figure S1. Schematic image of the structure. Infinite Bragg mirror infiltrated with quantum wells.

To obtain the dispersion equation for the eigenmodes of this structure we employ the transfer matrix technique[1]. General dispersion equation for the periodic structure can be given as

$$\cos(KD) = \frac{1}{2}\mathrm{Tr}(\hat{T}), \tag{1}$$

where $K$ is the Bloch wavevector, $D$ is the period of the structure, and $\hat{T}$ is the transfer matrix over the period of the structure. In the case of our structure, $\hat{T}$ can be written as a matrix product

$$\hat{T} = \hat{T}_{d_1/2}\hat{T}_{QW}\hat{T}_{d_1/2}\hat{T}_{d_2}, \tag{2}$$

where $\hat{T}_{d_1/2}$ is the transfer matrix for the propagation over the half of the first layer. Further on we assume the $s$-polarization of light (the electric field has no component, perpendicular to the layer interfaces). In this case the transfer matrix is given by

$$\hat{T}_{d_1/2} = \begin{pmatrix} \cos(k_{z1}d_1/2) & \frac{ik_0}{k_{z1}}\sin(k_{z1}d_1/2) \\ \frac{ik_{z1}}{k_0}\sin(k_{z1}d_1/2) & \cos(k_{z1}d_1/2) \end{pmatrix}, \tag{3}$$

where $k_0 = \omega/c$, and $k_{z1} = \sqrt{\varepsilon_1 k_0^2 - \mathbf{k}_\rho^2}$, and $\mathbf{k}_\rho = (k_x, k_y)$ is the in-plane wavevector component. The transfer matrix for the second layer is written in the completely analogous way.

The transfer matrix from the exciton quantum well can be written in the form

$$\hat{T}_{QW} = \begin{pmatrix} 1 & 0 \\ 2\frac{k_z r}{k_0 t} & 1 \end{pmatrix}, \tag{4}$$

where $r$ and $t$ are the reflection and transmission coefficients for the quantum well which in the case of the $s$ polarization are given by

$$r = \frac{i\sqrt{\varepsilon_1}k_0\Gamma_0/k_{z1}}{\omega_0' - \omega - i(\Gamma + \sqrt{\varepsilon_1}k_0\Gamma_0/k_{z1})}, \tag{5}$$

$$t = 1 + r, \tag{6}$$

where $\Gamma_0$ is the exciton radiative decay rate, $\omega_0'$ is the renormalized exciton frequency which in the approximation of infinitely thin QWs could be set equal to the exciton frequency $\omega_0$, and $\Gamma$ is the nonradiative exciton decay rate. Finally, we get the following dispersion equaiton:

$$\cos(KD) = \cos(k_{z1}d_1)\cos(k_{z2}d_2) - \frac{1}{2}\sin(k_{z1}d_1)\sin(k_{z2}d_2)\left(\frac{k_{z1}}{k_{z2}} + \frac{k_{z2}}{k_{z1}}\right)$$
$$- \frac{ir}{t}\left(\sin(k_{z1}d_1)\cos(k_{z2}d_2) + \sin(k_{z2}d_2)\left[\frac{k_{z1}}{k_{z2}}\cos^2(k_{z1}d_1/2) + \frac{k_{z2}}{k_{z1}}\sin^2(k_{z1}d_1/2)\right]\right). \tag{7}$$

This equation implicitly defines the polariton eigenfrequency $\omega(K, k_x, k_y)$. In the absence of losses, for the fixed value of $K$ and $k_\rho$ Eq. (7) has infinite number of solutions, corresponding to the infinite number of photonic bands in photonic crystal. We however focus at the four solutions, corresponding to the coupling of exciton to two photonic bands which have band centre frequencies closest to the exciton resonance. Dispersion of these four eigenmodes is shown in Fig. 1(b) in the manuscript.

## II. GROSS-PITAEVSKII EQUATION FOR BRAGG POLARITONS.

We examine only the lowest exciton-polariton branch. To derive the Gross-Pitaevskii equation for the polariton wave function, we introduce the kinetic energy operator

$$\hat{H}_0 = \hbar\omega(i\hbar\frac{\partial}{\partial z}, i\hbar\frac{\partial}{\partial x}, i\hbar\frac{\partial}{\partial y}). \tag{8}$$

The analytical expression for the kinetic energy operator is available only within the effective mass approximation, which holds for $k_\rho, K \ll \pi/D$.

In order to obtain the analytical expression for the kinetic energy operator of the polariton branch we first notice, that the lower polariton branch can be approximated as result of interaction of low photonic band and the exciton, since for the upper photonic branch, the electric field has nodes at the quantum well positions at the $\Gamma$ point. Thus, we first should obtain the kinetic energy operator for the lower photonic branch. This can be done, by setting $r = 0$ in Eq. (7) and expanding the equation in the vicinity of small $KD, k_xD, \omega/\omega_B$, where $\omega_B$ is the band gap centre satisfying the equation: $n_1d_1 + n_2d_2 = 2\pi c/\omega_B$. We then obtain the quadratic equation for the eigenfrequency $\omega$. The smaller solution corresponds to the lower photonic band

$$\omega_{ph} = \omega_B - \Omega_B + \frac{\hbar}{2m_{0\perp}}K^2 + \frac{\hbar}{2m_{0\parallel}}\left(k_x^2 + k_y^2\right), \tag{9}$$

where $\Omega_B$ is half of the band gap width:

$$\Omega_B = \frac{1}{2}\frac{\left|\frac{n_1d_1}{n_2d_2} - 1\right| |n_1 - n_2|}{(n_1 + n_2)}\omega_B, \tag{10}$$

and $m_{0\perp}, m_{0\parallel}$ are the orthogonal and lateral photonic effective masses which are given by

$$m_{0\perp} = -2\pi^2\hbar\Omega_B/(\omega_B^2 D^2), \tag{11}$$

$$m_{0\parallel} = \hbar\tilde{\varepsilon}\omega_B/c^2, \qquad \tilde{\varepsilon} = \frac{n_1^2 d_1 + n_2^2 d_2}{d_1 + d_2}. \tag{12}$$

We then can calculate the approximate polaritonic kinetic energy operator, assuming infinite exciton effecitve mass and assuming that the exciton frequency is at the frequency of photonic lower band edge. The polaritonic kinetic energy operator is then can be found from the eigenvalues of the following matrix:

$$\begin{pmatrix} \omega_{ph} & \Omega_P \\ \Omega_P & \omega_x \end{pmatrix}. \tag{13}$$

Diagonalization gives us the following kinetic energy operator:

$$\hat{H}_0 = \hbar\left(\omega_B - \Omega_B - \Omega_P + \frac{\hbar K^2}{2(2m_{0\perp})} + \frac{\hbar(k_x^2 + k_y^2)}{2(2m_{0\parallel})}\right). \tag{14}$$

We now obtain the Gross-Pitaevskii equation for the polariton branch. We account only for the lower polariton branch $\mathcal{P}_1$. The nonlinear term in the system Hamiltonian is given by

$$V_{nl} = \frac{6E_b\, a_b^3(D/d_{QW})}{V}\left(\frac{\Omega_p}{2\Omega_B}\right)^4 \sum_{k_1,k_2,q} \mathcal{P}^\dagger_{1,k_1+q}\mathcal{P}^\dagger_{1,k_2-q}\mathcal{P}_{1,k_1}\mathcal{P}_{1,k_2}$$
$$= \frac{\hbar g}{2}\sum_{k_1,k_2,q} \mathcal{P}^\dagger_{1,k_1+q}\mathcal{P}^\dagger_{1,k_2-q}\mathcal{P}_{1,k_1}\mathcal{P}_{1,k_2}. \tag{15}$$

Then, if in the reciprocal space nonlinear potential is wavevector independent, in the real space the potential is a delta-function $V_{nl}(|r-r'|) = g\delta(r-r')$.

We then introduce the bosonic operator

$$\hat{\Psi}_{\mathcal{P}_1}(r,t) = \sum_k \mathcal{P}_1(k) e^{ikr - i\omega_k t} \tag{16}$$

and write down the Heisenberg equation for this operator:

$$i\hbar \frac{\partial \Psi}{\partial t} = [\Psi, \hat{H}]. \tag{17}$$

We then exploit the commutation relations for the bosonic field operators:

$$[\Psi(r), \Psi^\dagger(r')] = \delta(r-r'). \tag{18}$$

The Hamiltonian of the system in the real space reads

$$\hat{H} = \int d^3r \Psi^\dagger(r) \hat{H}_0 \Psi(r) + \frac{\hbar g}{2} \int d^3r \Psi^\dagger_{\mathcal{P}_1}(r) \Psi^\dagger_{\mathcal{P}_1}(r) \Psi_{\mathcal{P}_1}(r) \Psi_{\mathcal{P}_1}(r). \tag{19}$$

We then apply the commutation relations to obtain

$$i\hbar \frac{\partial \hat{\Psi}_{\mathcal{P}_1}}{\partial t} = \hat{H}_{0\mathcal{P}_1} \hat{\Psi}_{\mathcal{P}_1} + \hbar g \hat{\Psi}^\dagger_{\mathcal{P}_1} \hat{\Psi}_{\mathcal{P}_1} \hat{\Psi}_{\mathcal{P}_1}. \tag{20}$$

Finally we assume that the there is a macroscopic occupation in the ground state of $\mathcal{P}_1$. Next, we use mean-field approach to replace corresponding polariton field operator $\hat{\Psi}(\mathbf{r})$ by its average value $\langle \hat{\Psi}(\mathbf{r}) \rangle \equiv \Psi(\mathbf{r})$, which characterizes the low branch polariton wave function[2]. We obtain a governing Gross-Pitaevskii equation for $\Psi(\mathbf{r})$

$$i \frac{\partial \Psi}{\partial t} = \left[ -\frac{\hbar}{2m_\parallel} \Delta_\parallel - \frac{\hbar}{2m_\perp} \frac{\partial^2}{\partial z^2} + g|\Psi|^2 \right] \Psi, \tag{21}$$

where $m_\parallel = 2m_{0\parallel}, \quad m_\perp = 2m_{0\perp}$.

[1] L.M. Brekhovskikh, *Waves in Layered Media* (Academic, New York, 1980).
[2] F. Dalfovo, S. Giorgini, L. P. Pitaevskii, and S. Stringari, Rev. Mod. Phys. **71**, 463 (1999).
